# Supplementary material for: Unveiling the BEC-droplet transition with Rayleigh superradiant scattering
Source: arXiv:2510.21211 source file (2026-09-26)
Supplement: Supplementary file 1 [file SM_SRdroplet_arXiv.tex]

\documentclass[aps,prl,twocolumn,superscriptaddress,english]{revtex4}

\usepackage{amssymb}
\usepackage{graphicx}
\usepackage{amsmath}
\usepackage{epsfig}
\usepackage{graphicx}% Include figure files
\usepackage{dcolumn}% Align table columns on decimal point
\usepackage{bm}% bold math
\usepackage[export]{adjustbox}

\usepackage{hyperref}% add hypertext capabilities
%\usepackage[mathlines]{lineno}% Enable numbering of text and display math
%\linenumbers\relax % Commence numbering lines

%\usepackage[showframe,%Uncomment any one of the following lines to test 
%%scale=0.7, marginratio={1:1, 2:3}, ignoreall,% default settings
%%text={7in,10in},centering,
%%margin=1.5in,
%%total={6.5in,8.75in}, top=1.2in, left=0.9in, includefoot,
%%height=10in,a5paper,hmargin={3cm,0.8in},
%]{geometry}
\usepackage{soul,ulem}
\usepackage[usenames,dvipsnames]{color}%Use color package
\usepackage{braket}

\begin{document}

\title{Supplementary Material for :\\Unveiling the BEC-droplet transition with Rayleigh superradiant scattering: }% Force line breaks with \\

\author{Mithilesh K. Parit}
\thanks{These authors contributed equally.}
\affiliation{Department of Physics, The Hong Kong University of Science and Technology, Clear Water Bay, Kowloon, Hong Kong, China}

\author{Mingchen Huang}
\thanks{These authors contributed equally.}
\affiliation{Department of Physics, The Hong Kong University of Science and Technology, Clear Water Bay, Kowloon, Hong Kong, China}

\author{Ziting Chen}
\affiliation{Department of Physics, The Hong Kong University of Science and Technology, Clear Water Bay, Kowloon, Hong Kong, China}

\author{Yifei He}
\affiliation{Department of Physics, The Hong Kong University of Science and Technology, Clear Water Bay, Kowloon, Hong Kong, China}

\author{Haoting Zhen}
\affiliation{Department of Physics, The Hong Kong University of Science and Technology, Clear Water Bay, Kowloon, Hong Kong, China}

\author{Gyu-Boong Jo}
\affiliation{Department of Physics and Astronomy, Rice University, Houston, TX, USA}%
\affiliation{Smalley-Curl Institute, Rice University, Houston, TX, USA}%
\affiliation{Department of Physics, The Hong Kong University of Science and Technology, Clear Water Bay, Kowloon, Hong Kong, China}

\date{\today}% It is always \today, today,
             %  but any date may be explicitly specified

\maketitle

\section{Experimental setup and procedure}

We prepare an ultracold gas of the $^{166}$Er isotope using a trapping and cooling scheme similar to that employed for $^{168}$Er \cite{ErMOT20, ErBEC23}. We load a crossed-ODT from a narrow-line MOT of $5 \times 10^7$ $^{166}$Er atoms at $T<20 \mu$K. Erbium MOT is loaded below the zero-crossing of the magnetic field due to the gravitational sag, and therefore atoms are spin-polarized to the lowest spin state $m_J = -6$ \cite{ErMOT20}. In our experiment, we define the $(x,y,z)-$coordinate system as follows: the vertical axis $z$ is aligned with gravity and the $x$ axis is along the horizontal ODT2 beam. Another horizontal ODT beam (ODT1) is perpendicular to ODT2 along the $y$ axis. These two ODT beams have beam waists of $w_{x-z}$ = 20 $\mu$ m and $w_{y-z}$ = 45 $\mu$ m, respectively. The magnetic dipole orientation follows the externally applied magnetic field, which is controlled by independently tuning the components $B_x$, $B_y$, and $B_z$ using three orthogonal pairs of bias coils. These pairs of coils define an orthonormal $(X, Y, Z)-$coordinate system with $Z = z$ and $(X, Y )$ rotated by an angle $\theta \approx 25.5^{\circ}$  relative to the $(x, y)$ plane. We have two imaging systems: one is a side-image along the $Y$ axis and the other is along the $Z$ axis.%\\

During evaporative cooling, we set the magnetic field to $B = 1.4 \ \text{G} \ \hat{z}$ and exponentially reduce the power of ODT1 and ODT2. At the end of the evaporation process, the measured trap frequencies are $(\omega_x, \omega_y, \omega_z) = 2\pi \times (209, 94, 205)$ Hz. A phase transition from a thermal gas to quantum degeneracy occurs around 160 nK, ultimately resulting in an almost pure Bose-Einstein condensate of approximately 50,000 atoms at 60 nK.

To prepare the trap for the BEC-droplet crossover, we adjust the trap geometry by increasing the power of ODT2 while simultaneously decreasing the power of ODT1 over a 50 ms interval. This reshaping changes the aspect ratio from $w_x / w_y = 2$ to 13. As a result, the final trap frequencies are $(\omega_x, \omega_y, \omega_z) = 2\pi \times (21, 290, 290)$ Hz. Meanwhile, to regulate the scattering length $a_s$, we gradually control the magnetic field amplitude from 1.4 G to 0.4 G, altering its direction from the $z$-axis to the $x$-axis aligned with the elongated ODT2 orientation. Over a 3 ms time interval, the magnetic field changes from 0.4 G to the target value, just before activating the SR pump beam. By varying the magnetic field amplitude, we tune the Rayleigh scattering rate to a maximum of 0.6 ms$^{-1}$, as determined through independent calibration. This modulation is crucial in significantly influencing the gain term (G) associated with superradiance. Following the superradiance process after TOF expansion, we count the ratio of recoiled atoms to the mother cloud for various Rayleigh scattering rates.

%------------------------------------
\subsection{Determination of three-body loss coefficient}
To determine the 3B loss coefficient ($L_3$) \cite{3B_loss}, we prepare a sample of thermal atom at 500 $\text{nK}$. We hold atoms from 0 to 2 seconds for different scattering lengths ($a_s$) and record the decay of atoms. The loss of thermal atoms with hold time, $t_h$ is given by 
\begin{equation}
    \frac{1}{N_{th}} \frac{d N_{th}}{dt_h}=-L_3^{th}\Bar{n}^2,
\end{equation}
where $N_{th}$, number of thermal atoms, is obtained by the Gaussian fitting and $\Bar{n}=\sqrt{\left<n^2\right>}$ is the mean square density of the thermal cloud. To describe the scaling of $\sqrt{\left<n^2\right>}$ with $N_{th}$, one can use prediction for an ideal gas at thermal equilibrium at temperature ($T$) whose state occupancies follow Boltzmann law. The $3B$ loss incurs the heating of the atoms. Therefore, taking into account the anti-evaporation effect one can derive $N_{th}$ as function $t_h$ as

\begin{equation}
    N_{th}\left( t_h \right)=\frac{N_0}{\left(1+3\gamma_0N_0^2 t_h \right)^{1/3}},
\end{equation}
where $N_0$ is initial atom number at $t_h=0~ms$. Now, $L_3^{th}$ is extracted from 

\begin{equation}
    L_3^{th}=\sqrt{27}\gamma_0 \left( \frac{2\pi k_BT}{m\Bar{\omega}^2} \right)^3,
\end{equation}
where $\Bar{\omega}=\left(\prod_{\eta=x, y, z} \omega_{\eta} \right)^{1/3}$. Finally, three-body coefficient $L_3$ of ${}^{166}$Er Bose gas is determined as $L_3=L_3^{th}/3!$, due to bosonization effect. The horizontal error bars are due to 5 $mG$ fluctuation in the magnetic field whereas error in $L_3$ comes from systematic error.

\begin{figure}%[ht]
    \includegraphics[width=8.0 cm, height=4.5 cm]{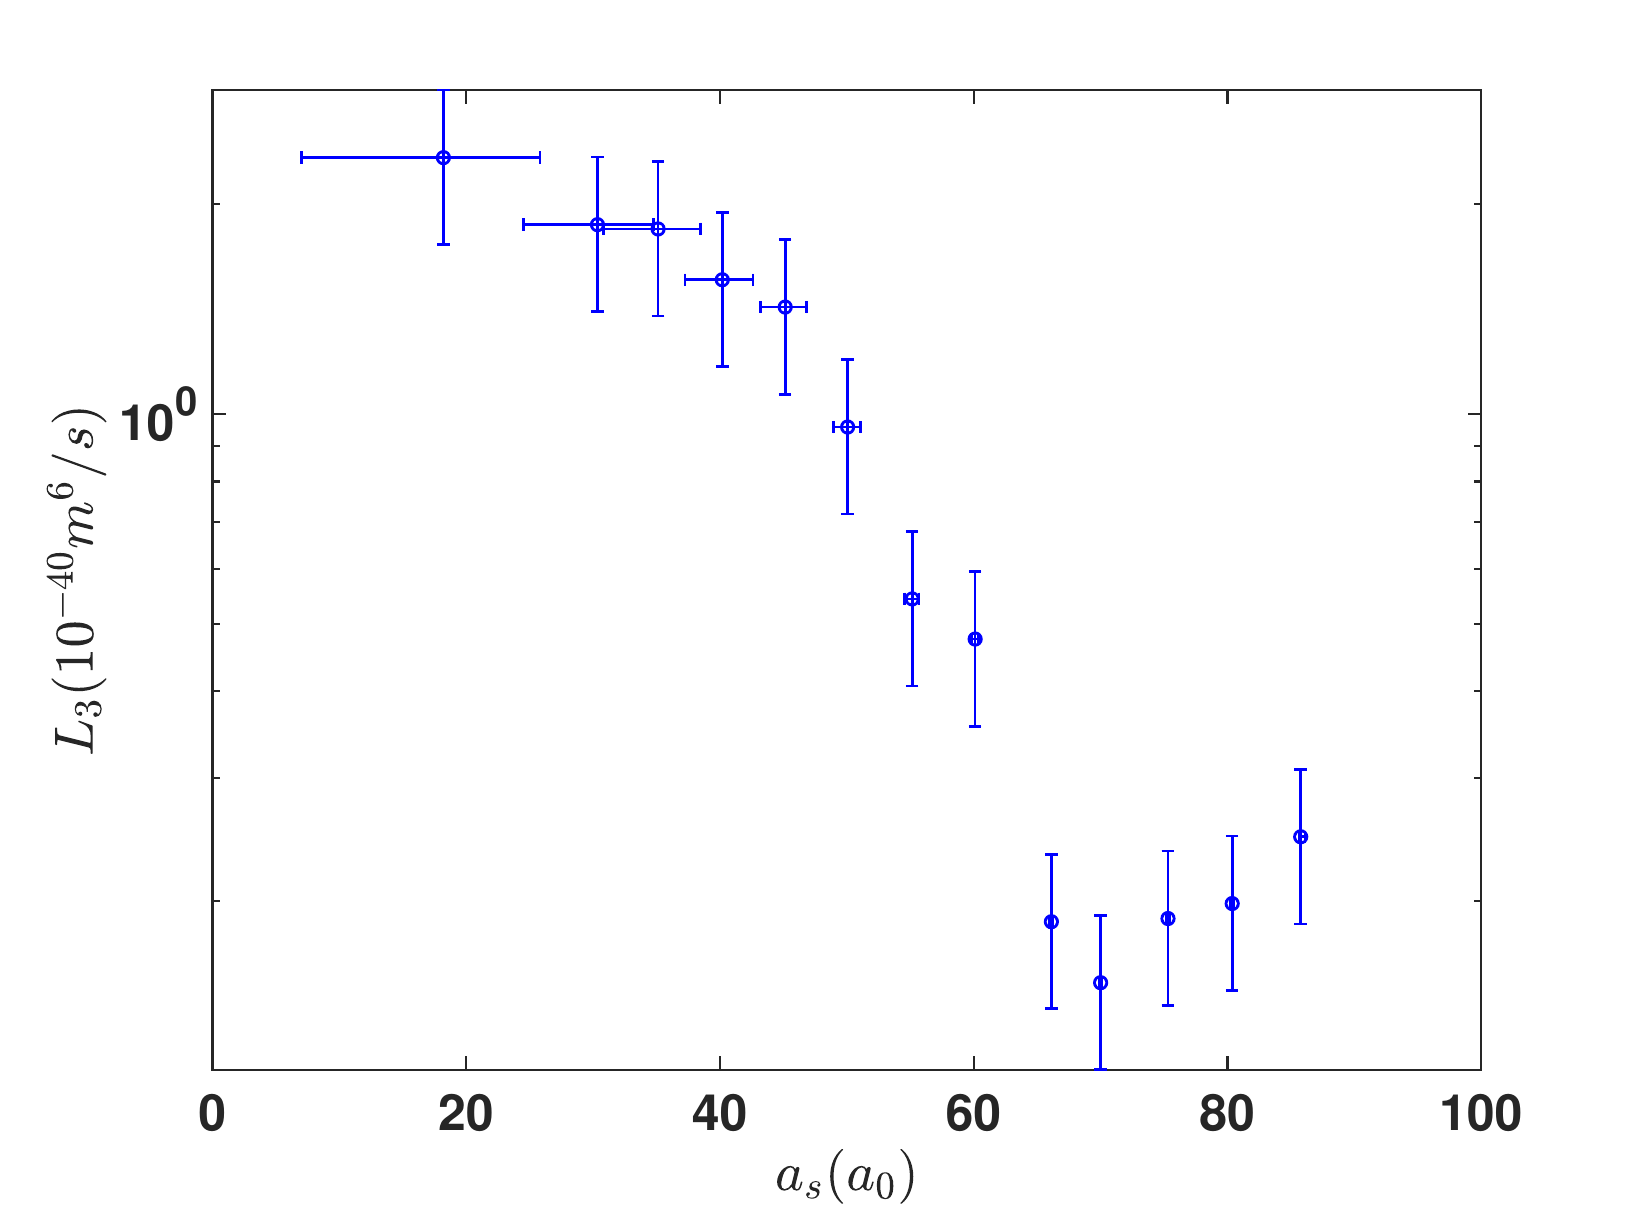}
    \caption{Measurement of three-body loss coefficient ($L_3$) of ${}^{166}$Er with respect to scattering length, $a_s$. See the text for the detailed explanation.}
 \label{fig_l3b}
\end{figure}
%\ \\

%------------------------------------
\subsection{Initial condensate atom number}

There is a significant 3B loss of atoms in the trap, with higher losses observed for lower $a_s$. Before activating the SR pump light, we ensure that the atom number is the same for all $a_s$. We control the atom number by adjusting the second evaporation time, which slightly affects the BEC fraction. In Fig. \ref{Ninitial}, we present the condensate number obtained by bimodal fitting of the total atomic cloud.

\begin{figure}[ht]
	\includegraphics[width=1.0\linewidth]{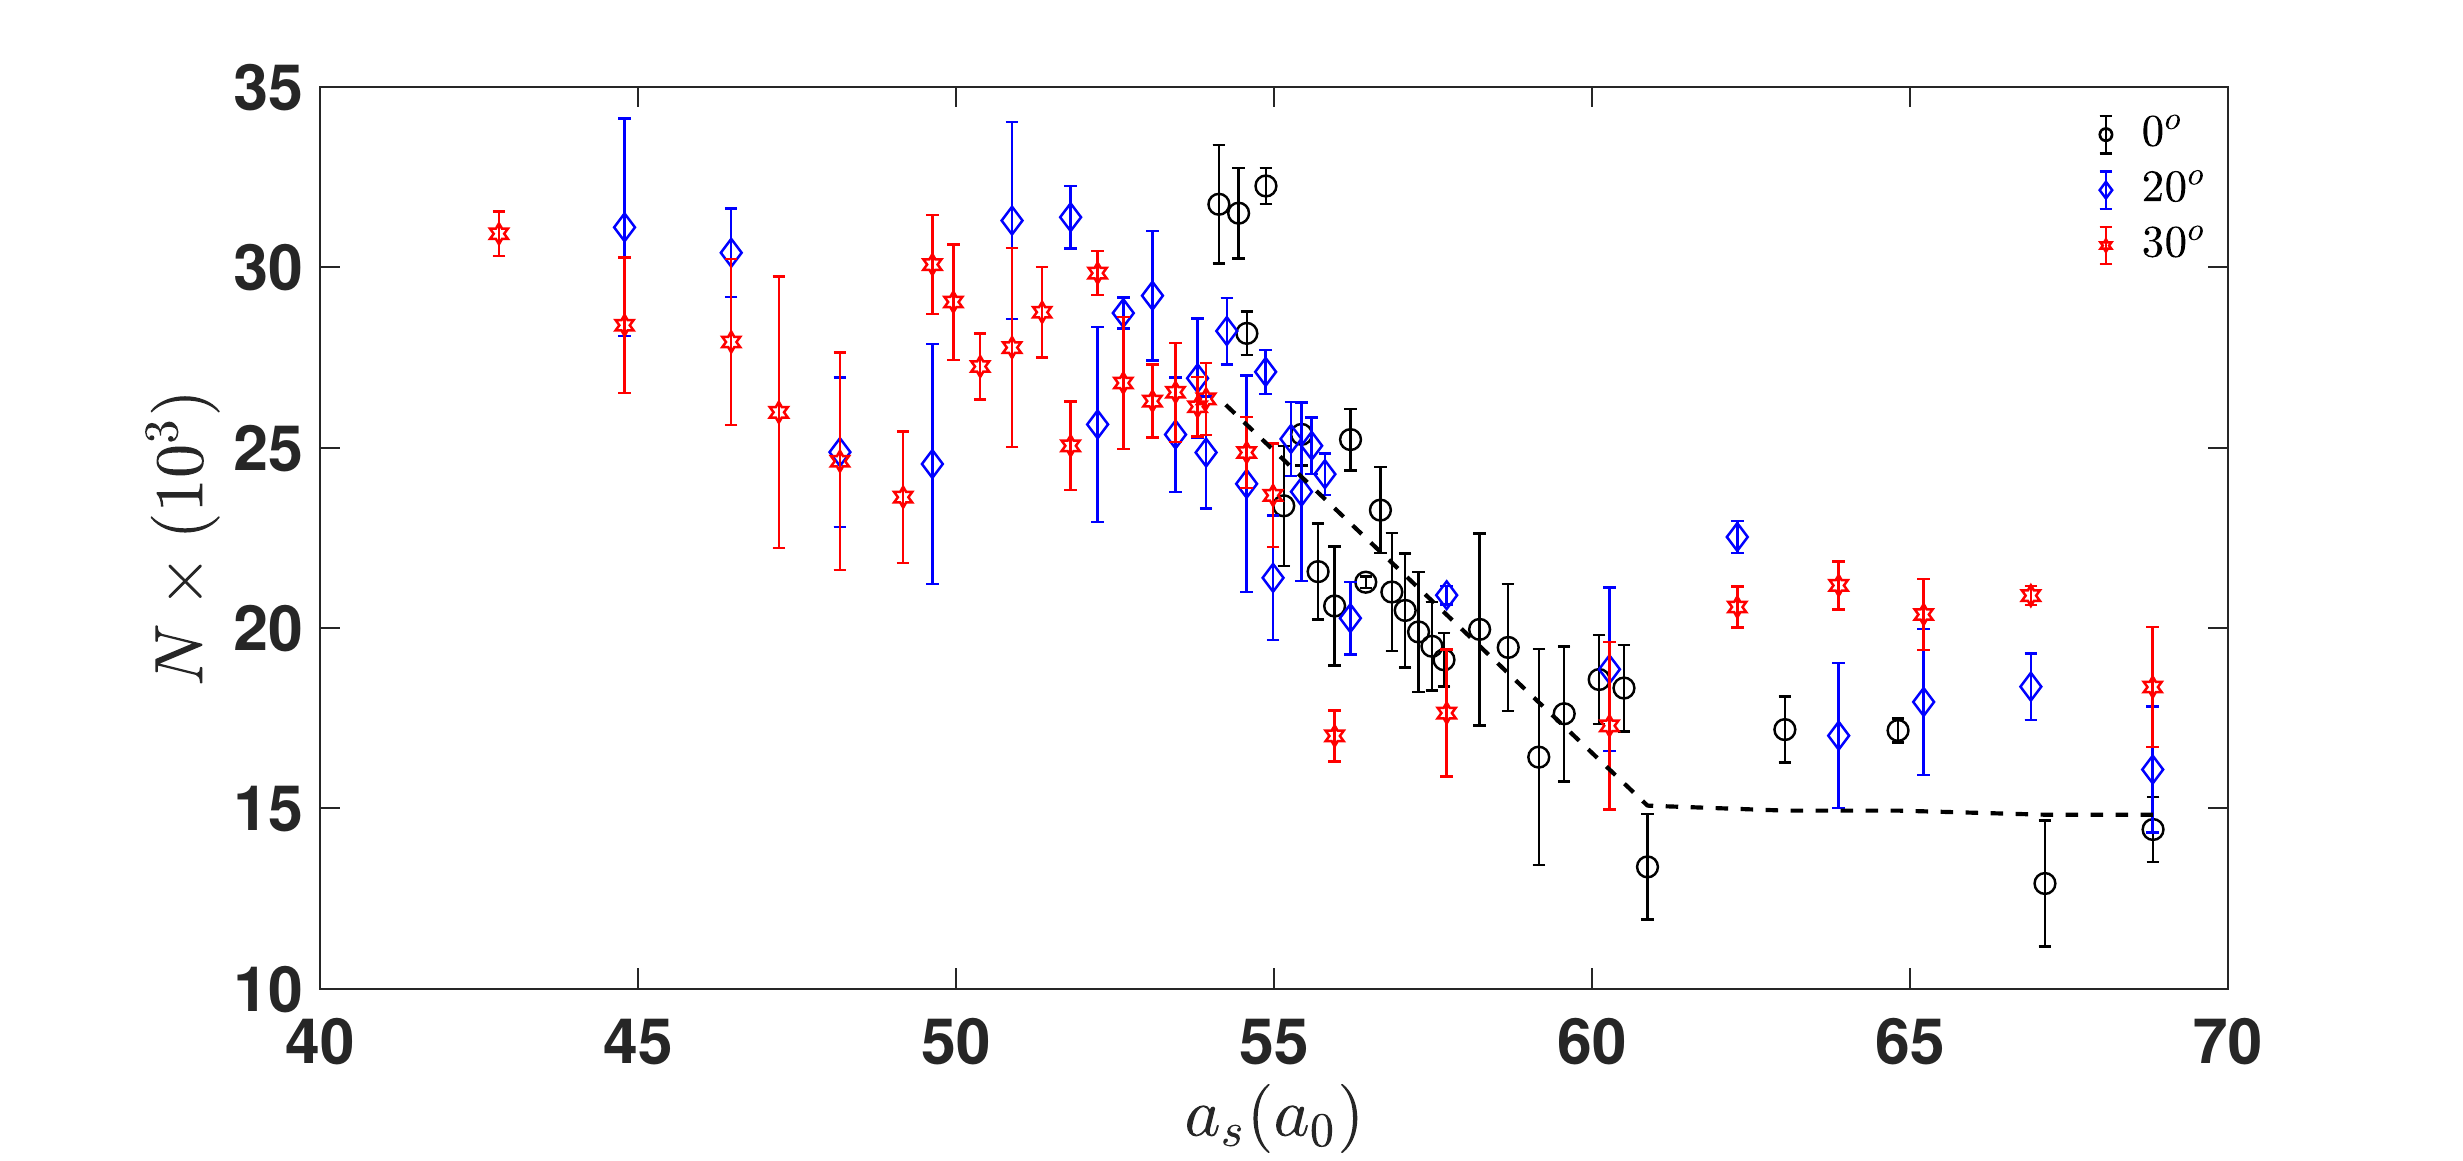}
    \caption{Condensate atom number for different dipolar orientations is measured just before quenching the magnetic field. The black dashed line is a guide for 0 degrees.}
 \label{Ninitial}
\end{figure}
%\ \\

%------------------------------------
\subsection{Expansion velocity measurement}
Following the quench of the magnetic field, we let the system evolve for $6~ms$ at the desired $a_s$ and abruptly switched off the ODT, allowing the free expansion of the cloud. We used the horizontal imaging system to quantify the expansion dynamics. The observed density distribution is fitted to a double Gaussian distribution function, from which the width ($\sigma_z$) along the z-axis is extracted. The width $\sigma_z$ is the size of central density. The size of the tail corresponds to the thermal fraction. It does not account for expansion velocity. We take data from $10$ to $17$ ms time of flight (TOF) to extract width, $\sigma_z$, of the cloud for each TOF. Finally, we fit $\sigma_z(t_{TOF)}$ to determine the expansion velocity, using the formula $\sigma_z(t_{TOF})=\sqrt{\sigma_{z,~0}^2+v_z^2 t_{TOF}^2}$. We vary $\epsilon_{dd}$ from $0.89$ to $1.57$ for three different angles. Upon increasing the $\epsilon_{dd}$, the expansion velocity reduces to a minimum value, $\approx 0.12~\mu m/ms$ for $\theta=0^o$.
Further increase of $\epsilon_{dd}$ results in the rapid expansion of the cloud, and expansion velocity begins to rise once again. With increasing dipolar orientation, we observe a clear shift of minimum expansion velocity towards larger $\epsilon_{dd}$. The observed shift in the minimum expansion velocity aligns well with the shift of the maximum portion of recoiled atoms, as illustrated in Fig.4(a) in the main text. The statistical error on expansion velocity is determined via relation $\Delta v_{exp}= \left( \Delta \sigma_z^{TOF}/\sigma_z^{TOF} \right) v_{exp}$. Here, we neglect the error on in-situ size of quantum droplets and $\Delta \sigma_z^{TOF}$ is obtained from size at TOF=17$~$ms.
%}

%%%%--------------------------------------------------------------------------------------
\section{Theoretical description}
In this section, we describe the calculation of phase-diagram and aspect ratio, based on time-dependent variational Gaussian ansatz \cite{PhaseCurv1997, Santos16a, Blakie16}. The underlying system is best described by the extended Gross-Pitaevaskii equation (eGPE), also known as generalized nonlocal nonlinear Schr\"{o}dinger equation \cite{Santos16b}. The eGPE includes external trap potential, short-range s-wave interaction, long-range dipolar interaction, and beyond mean-field quantum fluctuations, which is represented by
\begin{multline}
%\centering
    i\hbar \frac{\partial}{\partial t}\psi\left(\mathbf{r},~t\right)=\left[-\frac{\hbar^2\mathbf{\bigtriangledown}^2}{2m} + g\left|\psi\left(\mathbf{r},~t\right)\right|^2 + \mathbf{V}_{ext}\left(\mathbf{r},~t\right) \right.\\ \left. + \int \left|\psi\left(\mathbf{r'},~t\right)\right|^2\mathbf{U}_{dd}\left(\mathbf{r'-r}\right)d\mathbf{r'} + \right. \\ \left. \gamma\left(\epsilon_{dd}\right) \left|\psi\left(\mathbf{r},~t\right)\right|^3 - i\hbar \frac{L_3}{2} \left|\psi\left(\mathbf{r},~t\right)\right|^4 \right]\psi\left(\mathbf{r},~t\right).
    \label{eGPE}
\end{multline}
Here, the first and second terms refer to kinetic and mean-field energies, respectively, where $g=4\pi \hbar^2 a_{s}/m$. The third term, $\mathbf{V}_{ext}\left(\mathbf{r}\right)=\frac{1}{2}m\left(\omega_x^2 x^2 + \omega_y^2 y^2 + \omega_z^2 z^2 \right)$ is the external trap potential and $\mathbf{U}_{dd}\left(\mathbf{r'-r}\right)$ is the dipolar interaction potential, given by
\begin{eqnarray}
	U_{dd}(\mathbf{r})= \frac{\mu_0 {\mu}_{m}^2}{4\pi}~\frac{ 1 -3~\left(\hat{\bm e}_{{\mu}_{m}}\cdot \hat{\bm e}_{{r}}\right)^2 }{r^3},
	\label{DDI_gen_iden_dip}
\end{eqnarray}
where $\hat{\bm e}_{{m}}$ and $\hat{\bm e}_{{r}}$ are unit vectors, corresponding to $\bm{\mu}_{m}$ and $\bm r$. The second last term is first order beyond mean-field correction where $\gamma\left(\epsilon_{dd}\right)=\frac{32ga_s^{3/2}}{3\pi^{1/2}}F(\epsilon_{dd})$ with $\epsilon_{dd}=a_{dd}/a_s$ and $F(\epsilon_{dd})=\frac{1}{2} \int d\eta~ \text{sin}\left(\eta \right) \left[1+\epsilon_{dd}(3 \text{cos}^2\left(\eta \right))-1] \right]^{5/2}$ \cite{Santos16b, Pelster11, Pelster12}. In our experimental regime,  $F(\epsilon_{dd})=1+\frac{3}{2}\epsilon_{dd}^2$, true for all $\epsilon_{dd}\leq1.87$ in good approximation \cite{Blakie16}. The last term corresponds to three-body losses with $L_3$ as the loss coefficient \cite{3B_loss}. Hereafter (theory only), z-axis is considered as the axial direction.

%------------------------------------
\subsection{Gaussian variational ansatz}
We assume Gaussian ansatz as a variational solution to the eGPE \cite{PhaseCurv1997, Santos16a, QD16_FF},
\begin{equation}
    \psi\left(\mathbf{r},~t\right)=\sqrt{N(t)}~e^{i\phi(t)} ~\prod_{\eta=x, y, z} \frac{e^{-\left(\frac{\eta^2}{2\sigma_{\eta}^2} +i\eta^2\beta_{\eta}(t) \right)}}{\pi^{1/2}\sigma_{\eta}^{1/2}},
    \label{gva}
\end{equation}
where $\sigma_{\eta}$'s are variational parameters and the full widths at 1/e of the peak density. The Lagrangian density for the eGPE (Eq. \ref{eGPE}) is
\begin{multline}
    \mathcal{L}[ \psi]= \frac{i\hbar}{2}\left( \psi \frac{\partial \psi^*}{\partial t} -\psi^* \frac{\partial \psi}{\partial t} \right) +\frac{\hbar^2}{2m} \left| \mathbf{\bigtriangledown} \psi\right|^2 \\ + V_{ext}\left|\psi\right|^2+ \frac{g}{2} \left|\psi\right|^4  + \frac{2}{5} \gamma\left(\epsilon_{dd}\right) \left|\psi\right|^5\\ + \frac{1}{2} \int \mathbf{U}_{dd}\left(\mathbf{r', r}\right)\left|\psi\left(\mathbf{r'}\right)\right|^2 \left|\psi\left(\mathbf{r}\right)\right|^2d\mathbf{r'}.
    \label{lag_den}
\end{multline}
After obtaining the expression of $\mathcal{L}[ \psi]$ with Gaussian ansatz Eq. \ref{gva}, we use the Euler-Lagrange equations

\begin{equation}\label{Euler_Lag}
    \frac{d}{dt}\frac{\partial L}{\partial \dot{\lambda}}-\frac{\partial L}{\partial \lambda}=\int d^3 r \left[\Gamma \frac{\partial \psi^*}{\partial \lambda} + \Gamma^* \frac{\partial \psi}{\partial \lambda} \right],
\end{equation}
with Lagrangian, $L=\int d^3\mathbf{r} \mathcal{L}$ and $\Gamma=-i\hbar \frac{L_3}{2} \left|\psi\right|^4\psi$. Here, $\lambda$ stands for variational parameters, $N, ~\phi, ~\sigma_{\eta}$, and  $\beta_{\eta}$. After lengthy calculations, we get a set of differential equations

\begin{equation}
    \dot{N}=-\frac{3R}{\prod_{\eta}v_{\eta}^2}N^3
    \label{DE1}
\end{equation}

\begin{equation}
    \Ddot{v}_{\eta}=-v_{\eta} \left[\frac{7R^2N^4}{\prod_{\eta'}v_{\eta'}^4} +\frac{2RN^2}{\prod_{\eta'}v_{\eta'}^2} \sum_{\eta''\neq\eta}\frac{\dot{v}_{\eta''}}{v_{\eta''}} \right] - \frac{\partial U}{\partial v_{\eta}},
    \label{DE2}
\end{equation}
with potential %$U$

\begin{multline}
    U=\frac{1}{2}\sum_{\eta}\left[v_{\eta}^{-2} + \left( \frac{\omega_{\eta}}{\Bar{\omega}} \right)v_{\eta}^2 \right] + \frac{2}{3}\frac{PQN^{3/2}}{\left( \prod_{\eta}v_{\eta} \right)}\\ + \frac{PN}{\prod_{\eta}v_{\eta}} \left(1+\epsilon_{dd}F\left(\frac{\sigma_z}{\sigma_x}, \frac{\sigma_z}{\sigma_y}\right) \right),
    \label{pot_U}
\end{multline}
where
\begin{multline}
    F\left(k_x, k_y\right)=\frac{1}{4\pi}\int_{0}^{\pi}d\theta ~\text{sin}\theta \int_{0}^{2\pi} d\phi \\ \left( \frac{3~\text{cos}^2\theta}{\left(k_x^2 \text{cos}^2\phi + k_y^2 \text{sin}^2\phi\right)\text{sin}^2\theta + \text{cos}^2\theta} - 1\right)
    \label{dip_aniso_fn}
\end{multline}
is dipolar anisotropic function and $R=\frac{L_3}{\pi^3 3^{5/2}\Bar{\omega}\Bar{l}^6}$, $P=\sqrt{\frac{2}{\pi}}\frac{a}{\Bar{l}}$, and $Q=\frac{512 F(\epsilon_{dd})}{25\sqrt{5}\pi^{5/4}} \left(\frac{a}{\Bar{l}}\right)^{3/2}$. Through Eqs. (\ref{DE1})-(\ref{pot_U}), we have introduced the dimensionless parameters $\tau=\Bar{\omega}t$ and $\sigma_{\eta}=\Bar{l}v_{\eta}$ where $\Bar{l}=\sqrt{\hbar/m\Bar{\omega}}$ is the length of the oscillator and $\Bar{\omega}=\left(\prod \omega_{\eta} \right)^{1/3}$ is the geometric mean of the trap frequencies.

The initial condition for self-bound droplets is found by varying the variational parameters and creating a matrix of the potential $U$. Moreover, we consider the cylindrical symmetric external trap potential to calculate initial values, for which $\mathbf{V}_{ext}\left(\mathbf{r}\right)=\mathbf{V}_{ext}\left(\rho,~z\right)=\frac{1}{2}m\left( \omega_{\rho}^2\rho^2+\omega_z^2 z^2 \right)$ where $\rho^2=x^2+y^2$. Furthermore, we discover the ground state by locating the values of $\sigma_{\eta}=\Bar{l}v_{\eta}$ at the minimum of $U$. We fix atom number and scattering length to determine the variational parameters. To find the phase diagram of quantum droplets, we input $\omega_{\eta}=0$ and vary the scattering length, $a_s$. The value of $a_s$ at which $U=0$, is identified as the transition from BEC to the droplet for cigar-shaped traps.

\begin{figure}[ht]
\begin{center}
\includegraphics[width=8.0 cm, height=5.0 cm]{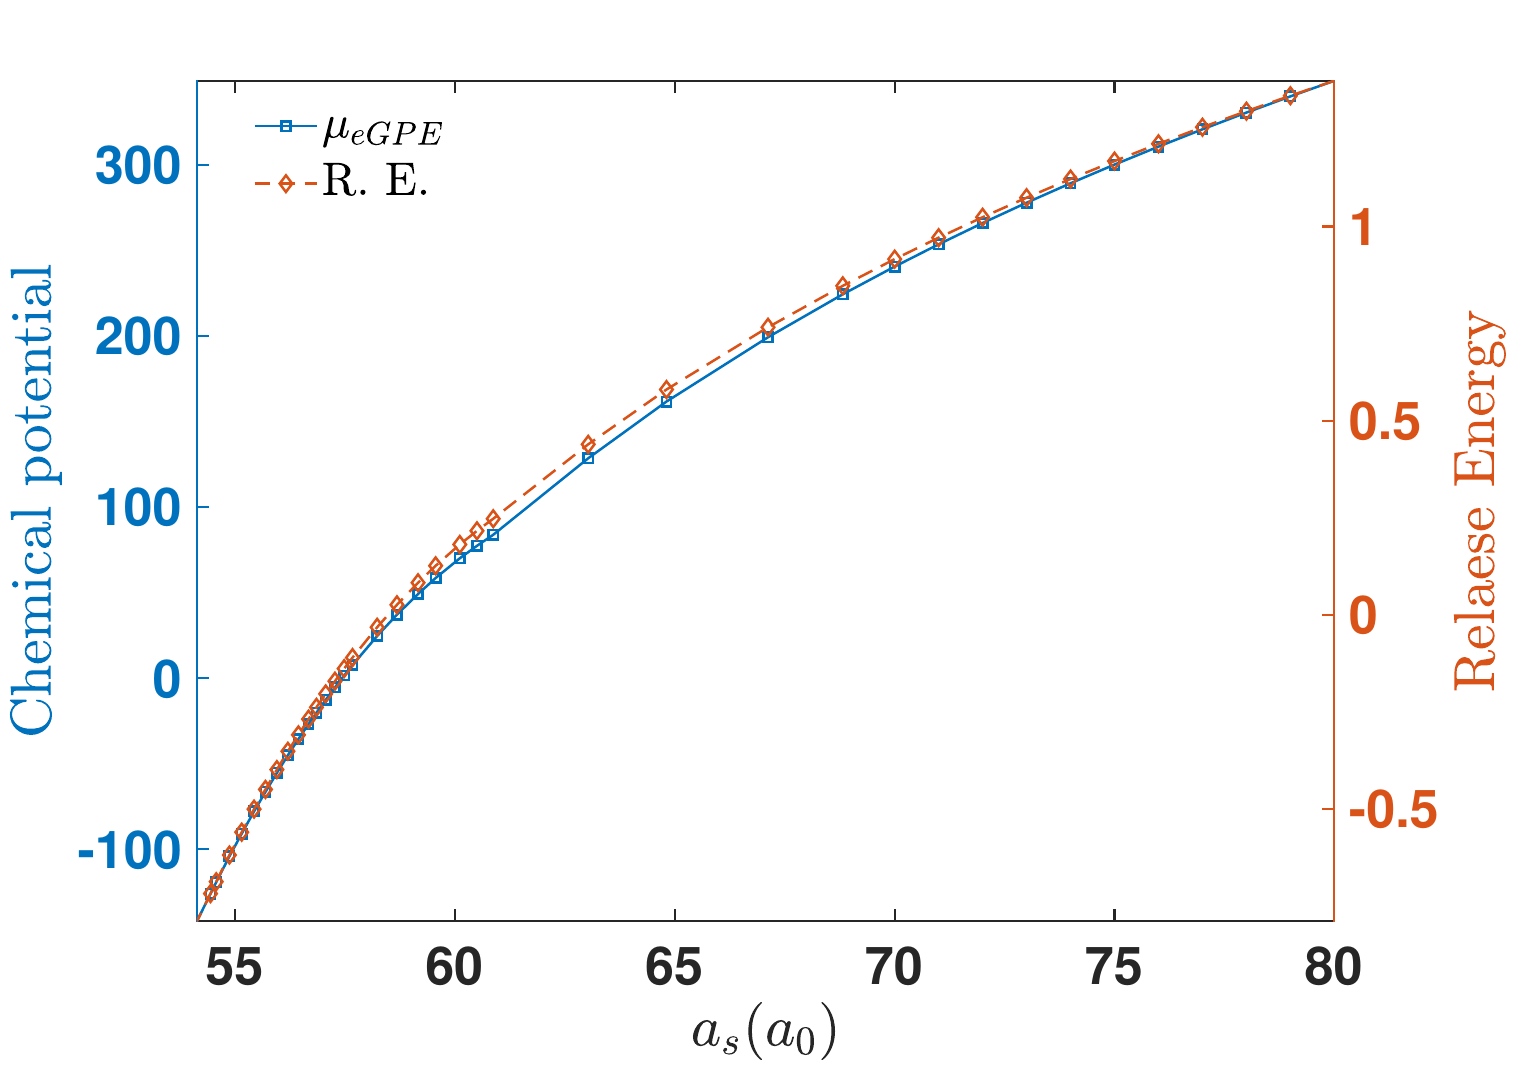}
\caption{Chemical potential and release energy of the system.}
\label{chem_pot_re}
\end{center}
\end{figure}

\subsection{Chemical potential and release energy} 
The analytical expression for chemical potential, $\mu=\frac{\partial E}{\partial N}$, can be obtained using eGPE (\ref{eGPE}) where the contribution to the energy comes from the MF, dipolar, and BMF interactions. It reads as
\begin{equation}
    E=E_{\text{s}}+E_{\text{dip}}+E_{\text{BMF}}.
    \label{Eq:RelEn}
\end{equation}
For Gaussian variation ansatz, Eq. \ref{gva}
\begin{align}\label{energy_mu1}
    E_s&=\frac{N^2g}{2\left(2\pi\right)^{3/2}\prod_{\eta}\sigma_{\eta}},\\[5pt]
    E_{dip}&=\frac{N^2g\epsilon_{dd}F\left(k_x, k_y\right)}{2\left(2\pi\right)^{3/2}\prod_{\eta}\sigma_{\eta}}, \\
    E_{BMF}&=\left(\frac{2N}{5}\right)^{5/2}\frac{\gamma\left(\epsilon_{dd}\right)}{\pi^{9/4}\prod_{\eta}\sigma_{\eta}^{3/2}},\label{energy_mu3}
\end{align}
where $\gamma\left(\epsilon_{dd}\right)$ and  $F\left(k_x, k_y\right)$ are defined above. In Fig. \ref{chem_pot_re}, chemical potential and release energy, $E_{\text{rel}}$ (per particle) are depicted as a function of target scattering length. Here plots are for $\mu \rightarrow \mu/h$ and $E_{\text{rel}} \rightarrow E/\left(N\hbar \Bar{\omega} \right)$.\\

\begin{figure}[ht!]
    \centering
    \includegraphics[width=0.9\linewidth]{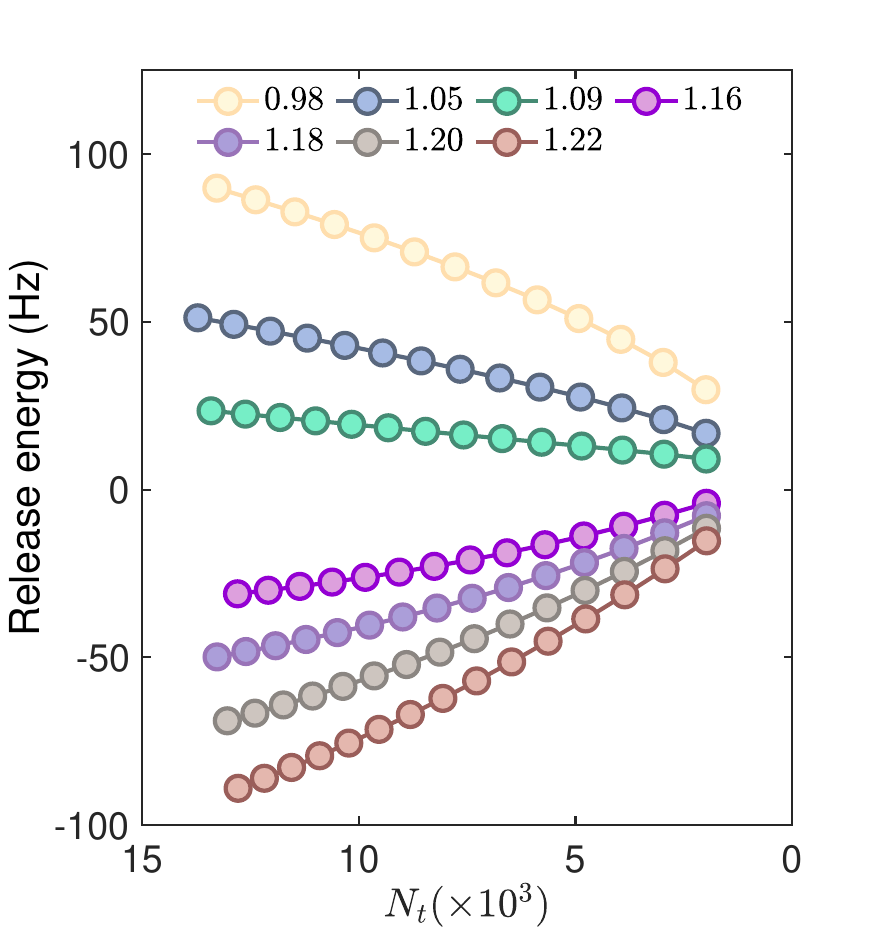}
    \caption{Release energy as a function of in-situ atom number at the end of quenching $a_s$.}
    \label{relaese_energy}   
\end{figure}

Interaction energy impacts the condensate property, including TOF expansion of the cloud. It has been utilized to infer the release energy of the system \cite{RE1, RE2}. Released energy depends on both the atom number and the final value of $a_s$. Furthermore, it provides insight into second-order coherence \cite{RE3}. In Fig. \ref{relaese_energy}, we present the released energy as a function of the atom number, which is analogous to the change in aspect ratio discussed in the main text.

%------------------------------------
\subsection{Phase diagram for BEC-droplet transition}
%------------------------------------
Ground-state phase diagram $-$ Here, the ground-state phase diagram for the BEC-droplet transition is obtained in the absence of the trap ($\mathbf{V}_{ext}\left(\mathbf{r},~t\right)=0$) using the effective potential $U$, Eq. \ref{pot_U} \cite{Santos16a}. This represents the self-bound solution that arises from the balance of underlying interactions. The curve indicates the point where $U$ vanishes for a given $\epsilon_{dd}$ and the atom number, N.

Phase diagram for a self-bound system based on release energy (in the main text)$-$ we use cylindrical symmetric trap geometry to calculate the phase diagram in the $a_s-\theta$ space for fixed N and in the $a_s-N$ space for fixed angle, where $\sigma_x=\sigma_r=\sigma_y$, thus $k_x=k_y=k$. For dipolar orientation $\theta$, it reduces to $F\left(k_x, k_y\right)=f(k)\left(\frac{1-3\text{cos}^2\theta}{2} \right)$ with
\begin{equation}
    f(k)=\frac{1+2k^2}{1-k^2}-\frac{3k^2 \text{arctanh}\left(\sqrt{1-k^2} \right) }{\left(1-k^2 \right)^{3/2}}.
\end{equation}

\end{document}
